# Supplementary material for: A Structured Method for Compilation of QAOA Circuits in Quantum Computing
Source: arXiv:2112.06143 source file (2022-07-20)
Supplement: Supplementary file 1 [file appendix.tex]

\clearpage
\onecolumn

{
\section*{Appendix}

We listed the major items we have revised according to the feedback from the reviewers. They are also highlighted in the paper.

\subsection*{1. Novelty} 
    \begin{itemize}
        \item We cited the two previous studies \cite{ogorman+:arxiv19, kivlichan+:prl18} that achieve linear solution for the line architecture. We described it in Section 3.1.  We also modified our introduction (Section 1) for an updated list of contributions, as well as our related work section to acknowledge that the line architecture solution is not new. 
        \item  We emphasize that the solution for Google sycamore architecture is new. We added detailed explanation for Sycamore. In particular, we show the challenges of handling odd-number row for the Sycamore architecture at Section 3.4.2. It cannot be trivially derived from the N*N grid solution.
        \item We emphasize the Maaps methodology with four condition is new. We added a new architecture -- the hexagon architecture to demonstrate how easy it is to come up with a solution with Maaps at Section 3.4.3. 
        \item We acknowledge that another concurrent study \cite{weidenfeller+:arxiv22} also comes up with a similar solution for 2D grid architecture. However, with an additional optimizations (Section 3.4.1), our work reduces 25\% of the depth. 
      
    \end{itemize}
    
\subsection*{2. Comparison with Tan}
\begin{itemize}
 \item In section 5.3, We added Table 3 showing a comparison with the QAOA-OLSQ by Tan \etal \cite{tan+:iccad20}. Due to the compilation overhead of QAOA-OLSQ, we cannot compare any circuit beyond 15 qubits. It takes over 2 days to compile a circuit with 15 qubits and density 40\% problem graph. We show the comparison for 10 qubits to 15 qubits. 
 \end{itemize}
 
 \subsection*{3. Heavy-hex correctness}
    \begin{itemize}
        \item We elaborated our solution for the IBM heavy-hex architecture in Section 3.5. It uses a bidirectional sweep to visit all nodes on the line embedding to guarantee the interaction between on-line and off-line nodes. We added additional figures as well. 
    \end{itemize}
\subsection*{4. Other modifications} 
\begin{itemize}
    \item We moved up the description for 2xN grid to Section 3.2. It is from our prior work in 2021. It is also a building unit in our Maaps method. We use it show we independently come up with the linear solution for grid, when it comes to comparison with the arXiv'22 paper by Weidenfeller \etal \cite{weidenfeller+:arxiv22}.
    \item We removed the terminology of Laaps throughout the paper. We did not highlight it as it is a small change.
\end{itemize}
    
}
